# Supplementary material for: Linear behavior of the optical conductivity and incoherent charge transport in BaCoS2
Source: arXiv:1712.01539 source file (2018-10-02)
Supplement: Supplementary file 1 [file supplemental_material.pdf]

# Supplemental material for the paper: Linear behavior of the optical conductivity and incoherent charge transport in BaCoS<sub>2</sub>

D. Santos-Cottin,<sup>1,2</sup> Y. Klein,<sup>3</sup> Ph. Werner,<sup>4</sup> T. Miyake,<sup>5</sup> L. de' Medici,<sup>1,2</sup> A. Gauzzi,<sup>3</sup> R. P. S. M. Lobo,<sup>1,2</sup> and M. Casula<sup>3</sup>

<sup>1</sup>*LPEM, ESPCI Paris, PSL University; CNRS; 10 rue Vauquelin, F-75005 Paris, France*

<sup>2</sup>*Sorbonne Université; CNRS; LPEM; F-75005 Paris, France*

<sup>3</sup>*Institut de Minéralogie, de Physique des Matériaux et de Cosmochimie (IMPMC), Sorbonne Université, CNRS UMR 7590, IRD UMR 206, MNHN; F-75252 Paris, France*

<sup>4</sup>*Department of Physics, University of Fribourg, 1700 Fribourg, Switzerland*

<sup>5</sup>*Research Center for Computational Design of Advanced Functional Materials, AIST, Tsukuba 305-8568, Japan*

## LDA CALCULATIONS

The LDA calculations have been performed with the Quantum Espresso [1] package. The geometry has been obtained from single crystal X-ray diffraction data at room temperature. These data were collected on an Oxford Diffraction Xcalibur-S four-circle diffractometer equipped with a Sapphire CCD-detector with  $Mo - K\alpha$  radiation ( $\lambda = 0.71073\text{\AA}$ , graphite monochromator) at 293 K. Data reduction, cell refinement, space group determination, scaling and analytical absorption correction [2] were performed using CrysAlisPro software. The structures were solved through Olex2 program [3], by the charge flipping algorithm. The refinement was then carried out with SHELXL [4] by full-matrix least-squares minimization and difference Fourier methods. All atoms were refined with anisotropic displacement parameters. We obtain a tetragonal high-temperature phase with the spacial point group  $P4/nmm$ . We report the coordinates of the 8 atoms in the tetragonal unit cell with  $a, b = 8.597876a_0$  and  $c/a = 1.957888$ . The atomic symbols are in the first column. The coordinates are in crystal units.

|    | x        | y        | z        |
|----|----------|----------|----------|
| Ba | 0.500000 | 0.000000 | 0.802560 |
| Ba | 0.000000 | 0.500000 | 0.197440 |
| Co | 0.500000 | 0.000000 | 0.407160 |
| Co | 0.000000 | 0.500000 | 0.592840 |
| S  | 0.500000 | 0.000000 | 0.151200 |
| S  | 0.000000 | 0.500000 | 0.848800 |
| S  | 0.000000 | 0.000000 | 0.500000 |
| S  | 0.500000 | 0.500000 | 0.500000 |

We used scalar relativistic pseudopotentials with non-linear core corrections for both Co and S atoms, while for Ba we utilized a relativistic separable dual-space Gaussian form [5]. The plane-wave cutoff has been set to 120 Ry. Convergence in the total energy is reached with an  $8 \times 8 \times 8$   $k$ -point grid, with a Gaussian smearing of 0.136 eV.

The tight-binding Hamiltonian used in subsequent DMFT calculations has been obtained with the Wannier90 code [6], using Co(3d) and S(3p) Wannier basis functions, an energy window of 15 eV, and a  $4 \times 4 \times 4$   $k$ -point grid. The agreement between the *ab initio* band structure and the one of the tight-binding model is very good, with a discrepancy  $< 30$  meV for all 22 bands over the whole  $k$ -space.

For optical conductivity calculations, we also derived a tight-binding Hamiltonian spanning a larger energy window (18 eV), to include empty Ba states, for a total of 34 Wannier orbitals. This has been generated by adding Ba(5s) and Ba(4d) Wannier states in the wannierization procedure, performed always on a  $4 \times 4 \times 4$   $k$ -mesh.

## cRPA CALCULATIONS

In the cRPA calculations, we evaluate the partially screened Hubbard interactions  $U$  and  $J$  acting on the Wannier  $d_i$  orbitals, defined as follows:

$$U_{ij} = \langle d_i d_j | W_r(0) | d_i d_j \rangle, \quad (1)$$

$$J_{ij} = \langle d_i d_j | W_r(0) | d_j d_i \rangle, \quad (2)$$

where  $W_r(\omega)$  is the partially screened Coulomb potential

$$W_r(\omega) = \frac{V}{1 - VP_r(\omega)}, \quad (3)$$

computed by excluding from the polarization  $P_r$  the screening channels that live in the low-energy manifold [7]. Hereafter, the  $d$  orbital order is  $i = \{z^2, xz, yz, x^2 - y^2, xy\}$ . The polarization  $P_r$  has been computed on a  $6 \times 6 \times 6$   $k$ -point grid, within the low-energy effective theory comprising both  $S(p)$  and  $Co(d)$  orbitals [8].

The  $U_{ij}^{\sigma,\sigma'}$  matrices obtained by cRPA for parallel ( $U^{\sigma,\sigma}$ ) and antiparallel ( $U^{\sigma,\bar{\sigma}}$ ) spin components are reported (in eV) in the following equations:

$$U_{ij}^{\sigma,\sigma} = U_{ij} = \begin{pmatrix} 3.714 & 2.848 & 2.848 & 2.328 & 2.386 \\ 2.848 & 3.946 & 2.589 & 2.581 & 2.648 \\ 2.848 & 2.589 & 3.946 & 2.581 & 2.648 \\ 2.328 & 2.581 & 2.581 & 4.023 & 3.214 \\ 2.386 & 2.648 & 2.648 & 3.214 & 4.161 \end{pmatrix}, \quad (4)$$

$$U_{ij}^{\sigma,\bar{\sigma}} = U_{ij} - J_{ij} = \begin{pmatrix} 0.000 & 2.366 & 2.366 & 1.582 & 1.610 \\ 2.366 & 0.000 & 1.907 & 1.876 & 1.940 \\ 2.366 & 1.907 & 0.000 & 1.876 & 1.940 \\ 1.582 & 1.876 & 1.876 & 0.000 & 2.763 \\ 1.610 & 1.940 & 1.940 & 2.763 & 0.000 \end{pmatrix}. \quad (5)$$

From the above matrices, we computed the spherical atomic averages  $U_{av} = 2.92$  eV and  $J_{av} = 0.90$  eV. From them, and with  $F_4$  obtained from Slater atomic ratios, we reconstruct the spherically symmetric  $U$  matrices, which read:

$$U_{\text{spherical}}^{\sigma,\sigma} = \begin{pmatrix} 3.957 & 2.978 & 2.978 & 2.356 & 2.356 \\ 2.978 & 3.957 & 2.564 & 2.564 & 2.564 \\ 2.978 & 2.564 & 3.957 & 2.564 & 2.564 \\ 2.356 & 2.564 & 2.564 & 3.957 & 3.185 \\ 2.356 & 2.564 & 2.564 & 3.185 & 3.957 \end{pmatrix}, \quad (6)$$

$$U_{\text{spherical}}^{\sigma,\bar{\sigma}} = \begin{pmatrix} 0.000 & 2.489 & 2.489 & 1.556 & 1.556 \\ 2.489 & 0.000 & 1.867 & 1.867 & 1.867 \\ 2.489 & 1.867 & 0.000 & 1.867 & 1.867 \\ 1.556 & 1.867 & 1.867 & 0.000 & 2.800 \\ 1.556 & 1.867 & 1.867 & 2.800 & 0.000 \end{pmatrix}. \quad (7)$$

The frequency dependence of the monopole interaction, obtained as the average over the diagonal matrix elements  $U(\omega) = \frac{1}{5} \sum_i \langle d_i d_i | W_r(\omega) | d_i d_i \rangle$ , is reported in Fig. 1. The frequency dependent part  $\mathcal{U}(\omega) = U(\omega) - U(0)$  is added to the spherically symmetric  $U$  matrices in Eqs. (6) and (7). This fully defines the retarded interactions used in our DMFT calculations.

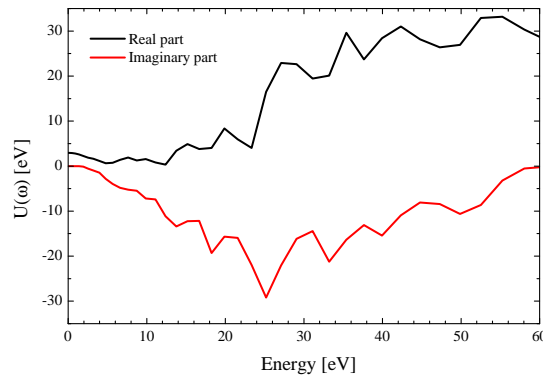

Figure 1: Frequency dependence of the partially screened  $U(\omega)$ .

## DMFT CALCULATIONS

We carried out DMFT calculations by using the CTQMC impurity solver for the  $d$  manifold with retarded interactions. The algorithm has been described in Refs. [9, 10].

By analytically continuing the self-energies on the real axis, we computed the  $k$ -resolved spectral function. In Fig. 2, we plot the orbital resolved spectral functions, obtained after  $k$ -integration and orbital projection of the  $k$ -resolved spectrum, for both static and dynamic  $U$ . Fig. 3 shows the imaginary part of the orbital resolved self-energies as a function of Matsubara frequencies.

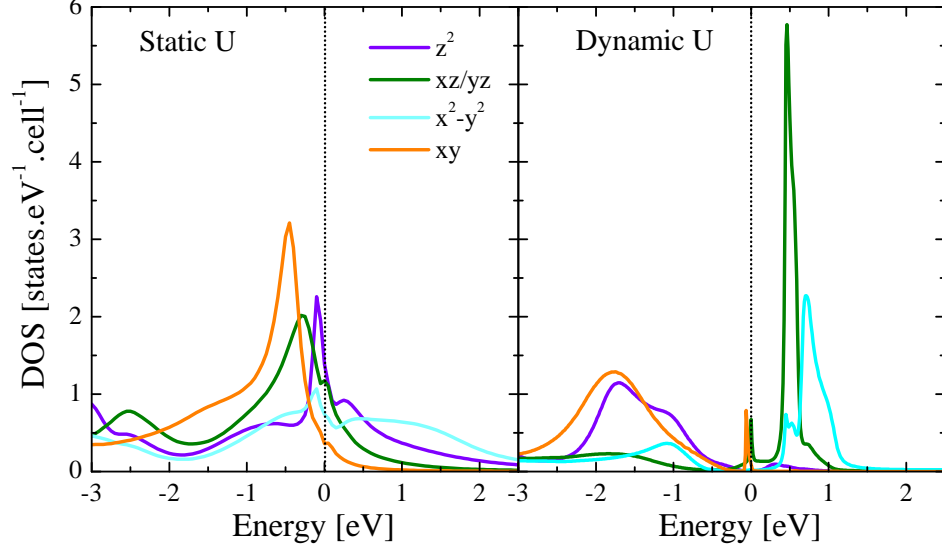

Figure 2: (color online) Projected density of states from LDA+DMFT with static (left panel) and dynamic (right panel)  $U$ .

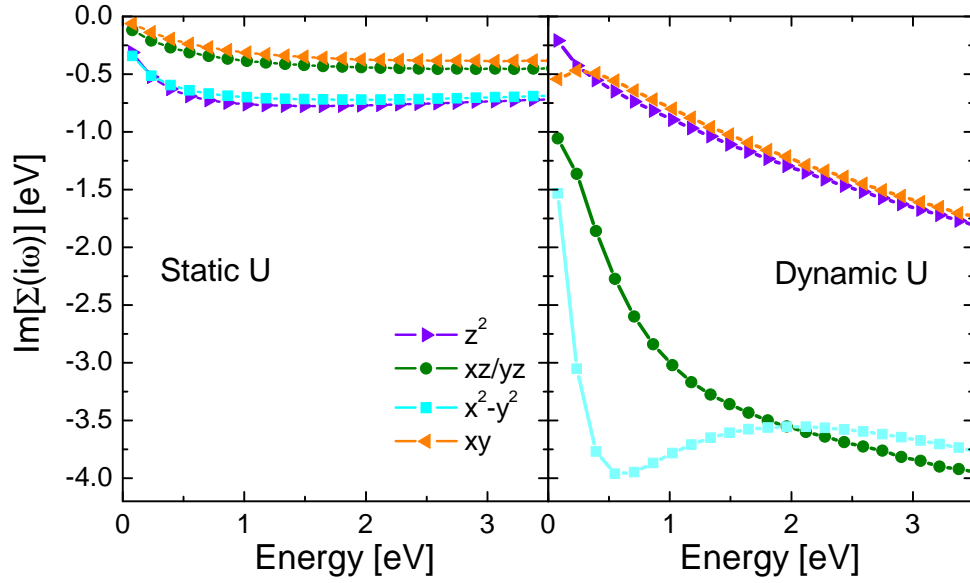

Figure 3: Imaginary part of the self-energies as a function of Matsubara frequencies from LDA+DMFT with static (left panel) and dynamic (right panel)  $U$ .

# VANISHING QUASI-PARTICLE-GAP MODEL

In order to understand the limitations and strengths of our *ab initio* calculations, we developed a simplified model for the DOS in Fig. 3 (c) of the main text, by parametrizing it as follows: (i) we keep the *ab initio* results ( $\rho_{ai}$ ) in the filled part below the charge gap and (ii) we replace the in-gap states at the Fermi level and the empty peaked structure by delta functions. The quasiparticle peak sits at a quasiparticle gap  $\Delta_1$  above  $\rho_{ai}$ . The second peak is placed at  $\Delta_2$  above the  $\rho_{ai}$  continuum and represents the underlying Mott-Hubbard gap. Thus, the effective model DOS becomes:

$$\rho_{eff}(\omega) = \rho_{ai}(\omega)\theta(-\omega) + c_1\delta(\omega - \Delta_1) + c_2\delta(\omega - \Delta_2), \quad (8)$$

where  $\theta$  is the Heaviside function. Additional broadening effects due to scattering processes are not included in the  $\delta$ -functions. The inset (b) in Fig. 4 shows a schematic representation of  $\rho_{eff}(\omega)$ . In the paramagnetic state, above 300 K, we set  $\Delta_1 = 0$  to reproduce a vanishing quasiparticle gap. Our best description of the data produces a Mott-Hubbard gap  $\Delta_2 = 75$  meV compatible with the thermal activated behavior of the resistivity. We computed the optical conductivity of this vanishing gap model through the current-current correlation function as a bubble diagram with renormalized quasiparticle Green's functions. We neglected the momentum dependence of the interband transition matrix elements, which considerably simplifies the optical conductivity expression, and we disregarded intraband transitions. Let us, for now, look only at the result for 320 K plotted in the main panel of Fig. 4, where the solid line is the experimental data and the dashed line our  $\rho_{eff}(\omega)$  calculations. As far as the low-energy slope is concerned, the agreement with the experiment is now excellent up to 0.2 eV, where the approximation of  $k$ -independent velocities breaks down. As calculations ignore the intraband transitions, the zero-frequency extrapolation of this model vanishes by construction. This model reveals that the value of the charge-transfer gap is of fundamental importance to reproduce the experimental linear behavior. It also shows that the *ab initio* results predict the proper DOS except for the Mott-Hubbard gap value, which is overestimated.

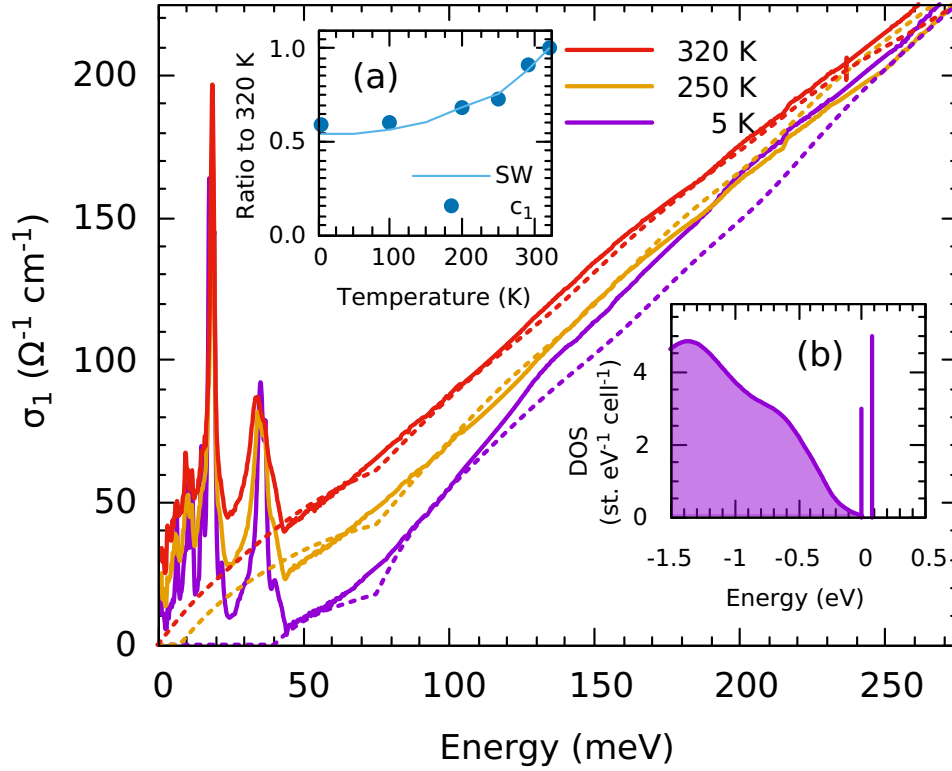

Figure 4: (color online) Experimental optical conductivity (solid lines) and  $\sigma(\omega)$  calculated from Eq. (8) disregarding intraband transitions, as described in the text. Inset (a) compares the temperature evolution of the  $c_1$  parameter (solid symbols) to the low frequency spectral weight, Eq. (1) in the main text, integrated to 50 meV (solid line). Both quantities are shown as a ratio to their values at 320 K. Inset (b) shows, schematically, the effective DOS utilized for the 320 K calculation.

This parametrization of the DOS also allows us to make an attempt at describing the antiferromagnetic optical response. Experimentally, the optical conductivity above and below the Néel temperature are not very different. The major distinction being the opening of a small low energy gap. This suggests that the Stoner mechanism can be applied to the in-gap states living

at  $\varepsilon_F$ , while the rest of the *ab initio*  $\rho(\omega)$  for the paramagnetic phase is preserved in the AF state. In order to describe this state, we took  $\Delta_1 = 40$  meV at 5 K [optical gap in Fig. 1(d) of the main text], and assumed that the  $\Delta_1$  gap varies linearly with temperature, closing at 300 K. Spectral weight conservation imposes  $c_1 + c_2$  to be a constant. Figure 4 (a) shows that the increase of  $c_1$  closely follows the low frequency optical spectral weight. With no further changes, this process describes the temperature dependence of  $\sigma_1(\omega)$ , as shown in the main panel of Fig. 4.

This toy model remarkably succeeds in reproducing the antiferromagnetic state, including the small dip close to  $\Delta_2$ , supporting the robustness of the *ab initio* calculations and strengthening the scenario of a vanishing charge-transfer gap.

- 
- [1] P. Giannozzi, S. Baroni, N. Bonini, M. Calandra, R. Car, C. Cavazzoni, D. Ceresoli, G. L. Chiarotti, M. Cococcioni, I. Dabo, et al., Journal of Physics: Condensed Matter **21**, 395502 (19pp) (2009).
  - [2] R. C. Clark and J. S. Reid, Acta Crystallographica Section A Foundations of Crystallography **51**, 887 (1995).
  - [3] O. V. Dolomanov, L. J. Bourhis, R. J. Gildea, J. A. K. Howard, and H. Puschmann, Journal of Applied Crystallography **42**, 339 (2009).
  - [4] G. M. Sheldrick, Acta Crystallographica Section A **64**, 112 (2008).
  - [5] C. Hartwigsen, S. Goedecker, and J. Hutter, Phys. Rev. B **58**, 3641 (1998).
  - [6] A. A. Mostofi, J. R. Yates, G. Pizzi, Y.-S. Lee, I. Souza, D. Vanderbilt, and N. Marzari, Computer Physics Communications **185**, 2309 (2014).
  - [7] F. Aryasetiawan, M. Imada, A. Georges, G. Kotliar, S. Biermann, and A. I. Lichtenstein, Phys. Rev. B **70**, 195104 (2004).
  - [8] T. Miyake and F. Aryasetiawan, Physical Review B **77**, 085122 (2008).
  - [9] E. Gull, A. J. Millis, A. I. Lichtenstein, A. N. Rubtsov, M. Troyer, and P. Werner, Rev. Mod. Phys. **83**, 349 (2011).
  - [10] P. Werner and M. Casula, Journal of Physics: Condensed Matter **28**, 383001 (2016).
